# Supplementary material for: Possible Spatial Correlation of Superconducting and Pseudogap Dynamics in a Bi-based Cuprate
Source: arXiv:2510.10906 ancillary file (2026-03-26)
Supplement: Supplementary file 1 [file S_SRLaBi.pdf]

# Supplemental Material for: Spatial Correlation of Superconducting and Pseudogap Dynamics in a Bi-based Cuprate

T. Shimizu,<sup>1</sup> T. Kurosawa,<sup>1</sup> S. Tsuchiya,<sup>1</sup> K. Yamane,<sup>1</sup> R. Morita,<sup>1</sup> Y. Toda,<sup>1</sup> and M. Oda<sup>2</sup>

<sup>1</sup>*Department of Applied Physics, Hokkaido University, Sapporo 060-8628, Japan.*

<sup>2</sup>*Department of Physics, Hokkaido University, Sapporo 060-0810, Japan.*

(Dated: October 9, 2025)

## I. ONE-DIMENSIONAL (1D) LINE SCANS OF $\Delta R/R$

One-dimensional line-scan measurements of  $\Delta R/R$  at  $T = 10$  K under different pump fluences are shown in Fig. S1. Along the dashed line indicated in Fig. 1(a) of the main text,  $\Delta R/R$  was measured at 43 positions with a spacing of  $\Delta x = 3.75 \mu\text{m}$  (total path length  $\sim 160 \mu\text{m}$ ) and is displayed as (upper) color density plots and (lower) transient traces. In the lower panels, the traces are vertically offset according to position. The  $\Delta R/R$  response is dominated by the superconducting component, characterized by a slow relaxation. From each transient trace, the superconducting response amplitude  $A_{\text{SC}}$  is defined as the time-averaged reflectivity change,  $\langle \Delta R/R \rangle_{2-10 \text{ ps}}$ , and is plotted in Fig. 2 of the main text. As seen in the color maps, the spatial intensity distribution remains weak under low excitation [Fig. S1(a)], whereas a pronounced distribution emerges under strong excitation [Fig. S1(c)]. This trend is consistent with the 2D  $\Delta R/R$  distributions shown in Figs. 1(c) and 1(d) of the main text.

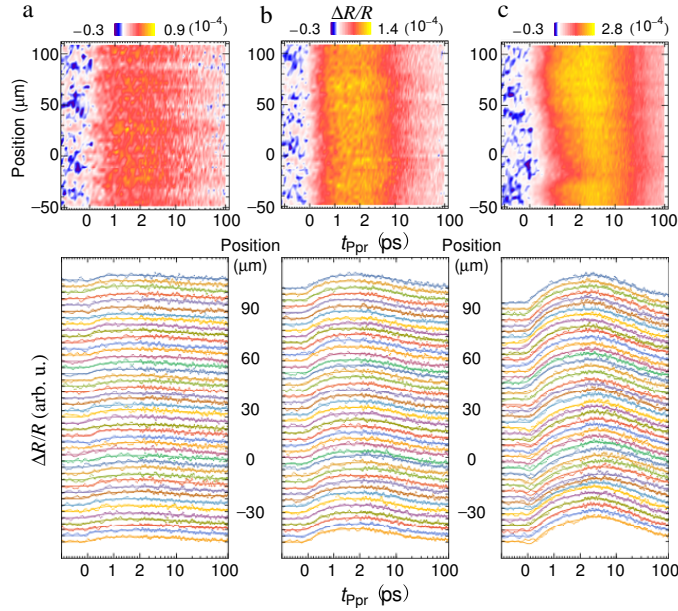

FIG. S1. 1D line scans of  $\Delta R/R$  obtained at  $T = 10$  K along the  $\sim 160 \mu\text{m}$  path indicated by the dashed line in Fig. 1(a) of the main text. The pump fluences are (a)  $\mathcal{F} = 0.6 \mu\text{J}/\text{cm}^2$ , (b)  $2.0 \mu\text{J}/\text{cm}^2$ , and (c)  $20 \mu\text{J}/\text{cm}^2$ . The upper panels display color density plots, while the lower panels show the corresponding  $\Delta R/R$  traces. Single-exponential fits to the data are shown as solid lines in the lower panels.

Figure S2 presents analogous line-scan measurements at  $T = 50$  K. The fast-decaying negative  $\Delta R/R$  corresponds to the pseudogap response. To emphasize this component, the time window of the horizontal axis is set to  $t_{\text{pr}} = -1$  to 6 ps (upper) and  $t_{\text{pr}} = -1$  to 10 ps (lower). Except under strong excitation, the pseudogap response nearly equilibrates within  $t_{\text{pr}} = 2$  ps. In contrast to the superconducting case, the pseudogap response exhibits a clear spatial distribution even under weak excitation. From these data, the pseudogap response amplitude  $A_{\text{PG}}$  is defined as  $-\langle \Delta R/R \rangle_{0.1-0.4 \text{ ps}}$  and plotted in Fig. 2 of the main text.

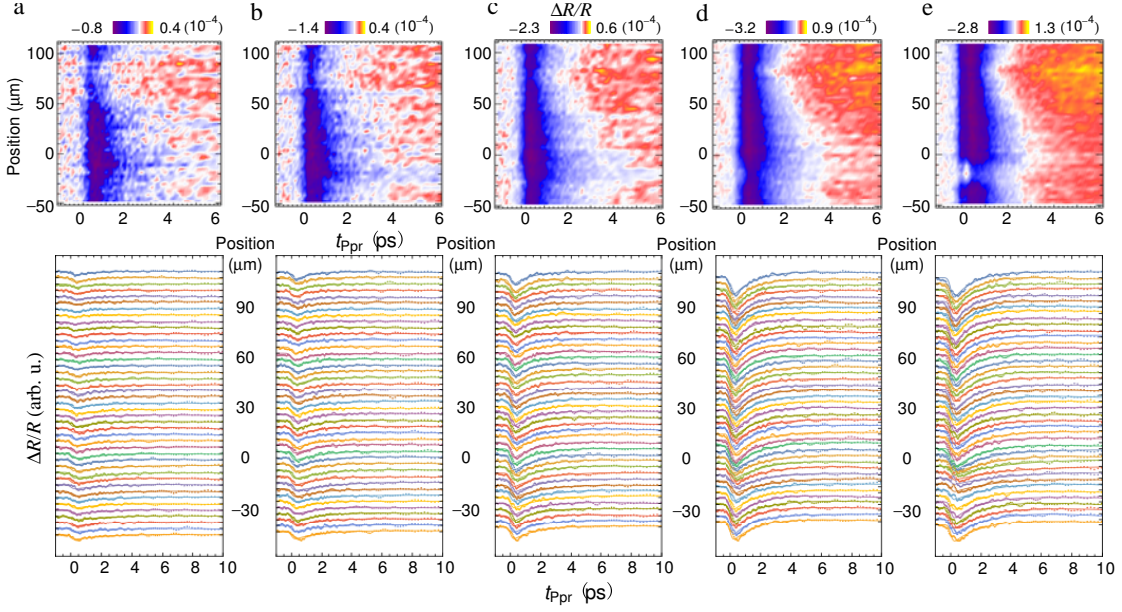

FIG. S2. The same as Fig.S2, but measured at  $T = 50$  K. The pump fluences are (a)  $5.2 \mu\text{J}/\text{cm}^2$ , (b)  $9.4 \mu\text{J}/\text{cm}^2$ , (c)  $20 \mu\text{J}/\text{cm}^2$ , (d)  $52 \mu\text{J}/\text{cm}^2$ , and (e)  $104 \mu\text{J}/\text{cm}^2$ .

## II. FLUENCE-DEPENDENT 1D DATA ANALYSIS USING A SATURATION MODEL

We first introduce the finite-penetration-depth excitation model for the fluence dependence of the transient reflectivity  $\Delta R/R$ . If the photoinduced change in the dielectric function  $\Delta\epsilon$  at the probe wavelength is described by a depth-dependent profile  $g(z)$ , then  $\Delta R/R$  can be evaluated as the integral of  $g(z)$  weighted by the exponential attenuation of the probe in the material. For coaxial Gaussian beams with finite diameters, this expression can be extended by an additional integration over the radial coordinate, where  $g(r, z)$  is obtained from an effective model that accounts for the spatial dependence of the excitation density:

$$U(r, z) = \mathcal{F}(1 - R_P)\alpha_P \exp\left[-\alpha_P z - \frac{2r^2}{\rho_P^2}\right], \quad (\text{S1})$$

where  $r$  is the radial distance from the beam center, and  $R_P$ ,  $\alpha_P$ , and  $\rho_P$  denote the pump reflectivity, absorption coefficient, and beam radius, respectively. Note that  $\Delta R/R$  in general depends not only on the static optical constants but also on an additional phase-shift term; while neglected here, a more accurate treatment including this term can be found in Ref. [1].

To account for the suppression of the SC (PG) state, which leads to a nonlinear excitation dependence of  $\Delta\epsilon$ , we adopt a simple phenomenological saturation model [1, 2]. In this model, the local amplitude of the transient dielectric function change,  $\Delta\epsilon(r, z) \propto g(r, z)$ , is approximated by a piecewise linear function of the locally absorbed energy density  $U(r, z)$ , with distinct slopes below and above  $U_{\text{th}}$ .

$$g(r, z) = h(U(r, z)),$$

$$h(u) = \begin{cases} \frac{u}{U_{\text{th}}}; & u < U_{\text{th}} \\ 1 + a(\frac{u}{U_{\text{th}}} - 1); & u \geq U_{\text{th}} \end{cases}. \quad (\text{S2})$$

Here,  $a$  denotes the relative slope in the normal state, and  $U_{\text{th}}$  is linked to the external threshold fluence through  $U_{\text{th}} = \mathcal{F}_{\text{th}}(1 - R_P)\alpha_P$ .

Next, we analyze the fluence dependence using the saturation model introduced above. Figures S3 and S4 present the fluence dependence of  $A_{\text{SC}} = \langle \Delta R/R \rangle_{2-10 \text{ ps}}$  and  $A_{\text{PG}} = -\langle \Delta R/R \rangle_{0.1-0.4 \text{ ps}}$ , respectively, obtained from Figs.S1 and S2. The data were acquired at 43 measurement points along a one-dimensional path of length  $\sim 160 \mu\text{m}$ . The solid lines represent best-fit curves based on the saturation model, and the corresponding saturation thresholds  $\mathcal{F}_{\text{th}}^{\text{SC,PG}}$  extracted from the fits are indicated in each panel. In all cases, clear saturation is evident. Note that the horizontal-

axis scales in Figs. S3 and S4 differ because of the distinct saturation thresholds of  $A_{SC}$  and  $A_{PG}$ . The extracted values of  $\mathcal{F}_{th}^{SC,PG}$  correspond to the results shown in Figs. 4(a) and (b) of the main text, respectively.

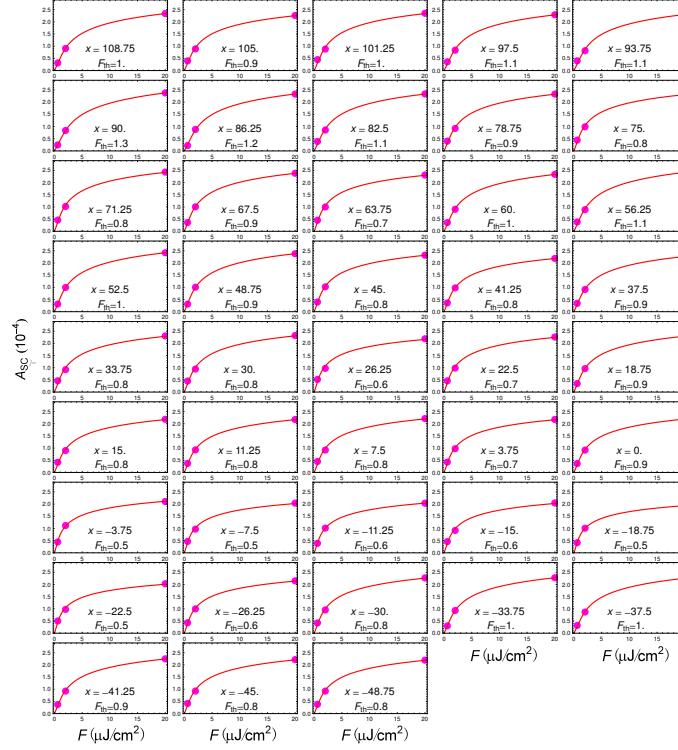

FIG. S3. Fluence dependence of  $A_{SC}$  obtained at  $T = 10$  K along the  $\sim 160 \mu\text{m}$  path indicated by the dashed line in Fig. 1(a) of the main text.  $A_{SC}$  values are extracted from the  $\Delta R/R$  traces in Fig. S1.

### III. TEMPERATURE DEPENDENCE OF $\Delta R/R$ AT TWO CHARACTERISTIC POSITIONS

In Fig. 1(b) and Fig. 3 of the main text, we compare representative  $\Delta R/R$  responses at two characteristic positions,  $P_A$  and  $P_B$ , marked by cross symbols in Fig. 1(b) of the main text. Figure S5 shows the temperature dependence of  $\Delta R/R$  at these locations.

Below  $T_c$ , the  $\Delta R/R$  signals originate from quasiparticle dynamics associated with superconductivity ( $\Delta R_{SC}/R$ ). A component with the opposite sign, attributed to the pseudogap ( $\Delta R_{PG}/R$ ), persists up to temperatures of about 200 K. At temperatures near room temperature, the  $\Delta R/R$  signal instead reflects electron-lattice relaxation in the metallic state ( $\Delta R_{ER}/R$ ). The identification of these components is well established in Bi-based cuprate superconductors [3–8].

Figures S5(a)-(d) present the temperature dependence of  $\Delta R/R$  under strong photoexcitation in the superconducting state ( $\mathcal{F}_{th}^{SC} < \mathcal{F} = 15 \mu\text{J}/\text{cm}^2 < \mathcal{F}_{th}^{PG}$ ). The upper panels show  $\Delta R/R$  at selected temperatures, while the lower panels display the corresponding color density plots. The warm-color regions dominating at low temperatures in Figs. S5(c) and (d) correspond to  $\Delta R_{SC}/R$ , while the cold-color regions correspond to  $\Delta R_{PG}/R$ . The temperature range  $T_c < T < 40$  K reflects the presence of superconducting fluctuations. The values of  $A_{PG}$  in Fig. 3(d) of the main text are derived from the data at  $T > 40$  K, excluding the region affected by superconducting fluctuations in Figs. S5(c) and (d).

In contrast, Figs. S5(e) and (f) show results under weak excitation ( $\mathcal{F}_{th}^{SC} \approx \mathcal{F} = 1.1 \mu\text{J}/\text{cm}^2$ ), where only the quasiparticle response associated with superconductivity is observed. The  $A_{SC}$  in Fig. 3(c) of the main text is derived from the data at  $T < 45$  K shown in Figs. S5(e) and (f).

A comparison between Figs. S5(a) and S5(b) reveals that the magnitude of  $\Delta R_{PG}/R$  at  $P_B$  (blue curves) exceeds that at  $P_A$ , which in turn affects the rise time of  $\Delta R/R$  below  $T_c$ . This effect is also evident in the color density plots: in Fig. S5(d), the blue region associated with  $\Delta R_{PG}/R$  extends to lower temperatures below  $T_c$  compared with Fig. S5(c).

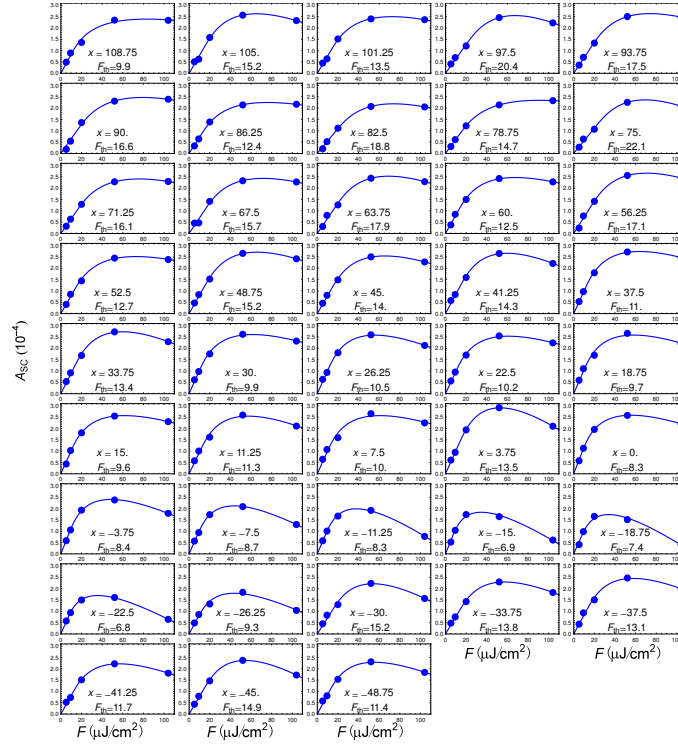

FIG. S4. Fluence dependence of  $A_{PG}$  obtained at  $T = 50$  K along the  $\sim 160$   $\mu\text{m}$  path indicated by the dashed line in Fig. 1(a) of the main text.  $A_{PG}$  values are extracted from the  $\Delta R/R$  traces in Fig. S2.

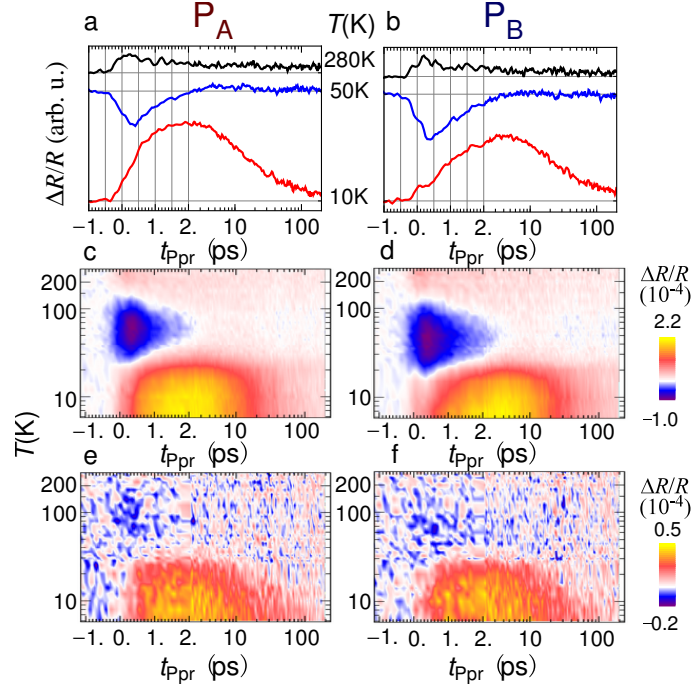

FIG. S5. Temperature dependence of the transient reflectivity at (left)  $P_A$  and (right)  $P_B$ . (a, b)  $\Delta R/R$  at selected  $T$  with a pump fluence of  $\mathcal{F} = 15 \mu\text{J}/\text{cm}^2$ . These two results are shown together in Fig. 1(b) of the main text. For clarity,  $\Delta R/R$  at different temperatures are vertically offset. (c, d) Corresponding color density plots of  $\Delta R/R$  as a function of time and temperature at  $\mathcal{F} = 15 \mu\text{J}/\text{cm}^2$ . (e, f) Same as (c, d) but at reduced pump fluence of  $\mathcal{F} = 1.1 \mu\text{J}/\text{cm}^2$ .

#### IV. FLUENCE DEPENDENCE OF $\Delta R/R$ AT TWO CHARACTERISTIC POSITIONS

Figure S6 presents the fluence ( $\mathcal{F}$ ) dependence of  $\Delta R/R$  at positions  $P_A$  and  $P_B$ . The upper panels (Figs. S6 (a) and (b)) show data taken below  $T_c$  ( $T = 10$  K), while the lower panels (Figs. S6 (c) and (d)) show data above  $T_c$  ( $T = 40$  K). In all cases, clear saturation in  $\Delta R/R$  is observed, indicative of photoinduced phase destruction of the SC ( $\Delta R_{SC}/R$ ) and PG ( $\Delta R_{PG}/R$ ) components. The peak shift of  $\Delta R/R$  with increasing fluence in Figs. S6 (a) and S6 (b) arises from the enhancement of  $\Delta R_{PG}/R$ , while  $\Delta R_{SC}/R$  remains nearly constant in the saturated regime. Since  $\Delta R_{PG}/R$  exhibits a higher threshold fluence for photoinduced phase destruction than  $\Delta R_{SC}/R$ , the  $\Delta R_{PG}/R$  component, having the opposite sign to  $\Delta R_{SC}/R$ , becomes dominant at fluence exceeding the superconducting threshold, thereby causing the observed peak shift in  $\Delta R/R$ .

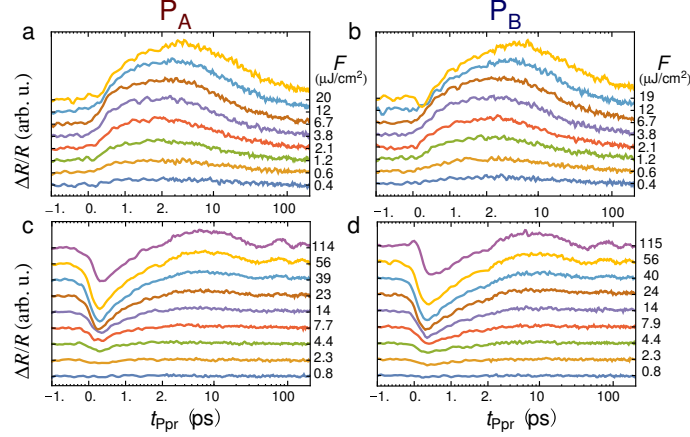

FIG. S6. Fluence dependence of the transient reflectivity at (left)  $P_A$  and (right)  $P_B$ . (a, b)  $\Delta R/R$  at selected  $\mathcal{F}$  at  $T = 10$  K, and at (c,d)  $T = 40$  K. For clarity, the traces at different fluences are vertically offset.

- 
- [1] M. Naseska, A. Pogrebna, G. Cao, Z. A. Xu, D. Mihailovic, and T. Mertelj, Phys. Rev. B **98**, 035148 (2018), URL <https://link.aps.org/doi/10.1103/PhysRevB.98.035148>.
  - [2] P. Kusar, V. V. Kabanov, S. Sugai, J. Demsar, T. Mertelj, and D. Mihailovic, Phys. Rev. Lett. **101**, 227001 (2008), URL <https://link.aps.org/doi/10.1103/PhysRevLett.101.227001>.
  - [3] Y. H. Liu, Y. Toda, K. Shimatake, N. Momono, M. Oda, and M. Ido, Phys. Rev. Lett. **101**, 137003 (2008), URL <https://link.aps.org/doi/10.1103/PhysRevLett.101.137003>.
  - [4] C. Giannetti, F. Cilento, S. Dal Conte, G. Coslovich, G. Ferrini, H. Molegraaf, M. Raichle, R. Liang, H. Eisaki, M. Greven, et al., Nature Communications **2**, 353 (2011).
  - [5] Y. Toda, T. Mertelj, P. Kusar, T. Kurosawa, M. Oda, M. Ido, and D. Mihailovic, Physical Review B **84**, 174516 (2011).
  - [6] G. Coslovich, C. Giannetti, F. Cilento, S. Dal Conte, T. Abebaw, D. Bossini, G. Ferrini, H. Eisaki, M. Greven, A. Damascelli, et al., Physical Review Letters **110**, 107003 (2013).
  - [7] Y. Toda, F. Kawanokami, T. Kurosawa, M. Oda, I. Madan, T. Mertelj, V. V. Kabanov, and D. Mihailovic, Phys. Rev. B **90**, 094513 (2014).
  - [8] T. Akiba, Y. Toda, S. Tsuchiya, M. Oda, T. Kurosawa, D. Mihailovic, and T. Mertelj, Phys. Rev. B **109**, 014503 (2024), URL <https://link.aps.org/doi/10.1103/PhysRevB.109.014503>.
